# Supplementary material for: Reversing the cycle: self-supervised deep stereo through enhanced monocular distillation
Source: arXiv:2008.07130 source file (2020-08-17)
Supplement: Supplementary file 1 [file eval_ustereo_supp.tex]

%-------------------------------------------------------------------------
% KITTI 2015 test
%-------------------------------------------------------------------------

\begin{table*}[!htbp]
\centering
\scalebox{0.65}{
\begin{tabular}{l|c|cc|cccc|ccc}
\multicolumn{5}{c}{} &\multicolumn{2}{c}{\cellcolor{blue!25} Lower is better}
 & \multicolumn{2}{c}{\cellcolor{LightCyan} Higher is better} \\
\hline
Method & Region & GT & Pre-train  & \cellcolor{blue!25} RMSE & \cellcolor{blue!25} RMSE log & \cellcolor{blue!25} \textbf{D1 (\%) \textcolor{red}{$\downarrow$}} & \cellcolor{blue!25} EPE &  \cellcolor{LightCyan}$\delta<$1.25 &  \cellcolor{LightCyan}$\delta<1.25^2$ & \cellcolor{LightCyan}$\delta<1.25^3$ \\
\hline

\hline
Pilzer et al. \cite{pilzer2018unsupervised} & Noc & & & (6.005) & (0.205) & (29.106) & (3.061) & (0.852) & (0.947) & (0.979) \\
Godard et al.\cite{Godard_CVPR_2017} (stereo) & Noc & & & 4.392 & 0.146 & 9.19 & - & 0.942 & 0.978 & 0.989\\
Yang et al.\cite{yang2018segstereo} & Noc  & & & - & - & 8.95 & 1.61 & - & - & -\\
Tonioni et al. \cite{Tonioni_2017_ICCV} & &  & - & - & 8.51 & 1.48 & - & - & -\\
Zhou et al.\cite{Zhou_2017_ICCV} & Noc  & & & - & - & 8.35 & 1.44 & - & -\\
Lai et al.\cite{lai19cvpr} & Noc & & & 4.168 & 0.149 &  8.22 & 1.40 & 0.947 & 0.979 & 0.990\\
Yang et al.\cite{yang2018segstereo} & Noc  & & \checkmark & - & - & 7.70 & 1.46 & - & - & -\\
Li and Yuan \cite{Li2018OcclusionAS} & Noc  & & \checkmark & - & - & 6.65 & 1.73 & - & - & -\\
\textbf{Ours} (\stereodepth) \textdagger & Noc & & &  3.894 &  0.116 &  4.21 & 1.06 & 0.971 &  0.988 &  0.993 \\
\textbf{Ours} (\psm ) & Noc  & & &  3.772 & 0.115 & 3.68 &      0.99 &  0.974 & 0.988 & 0.993 \\
\textbf{Ours} (\iresnet ) & Noc  & & & 3.472 & 0.107 & 3.64 &  0.99 & 0.975 & 0.989 & 0.994 \\
\textbf{Ours} (GwcNet \cite{guo2019group}) & Noc & & & 3.623 & 0.111 & 3.78 & 1.02 & 0.974 & 0.989 & 0.993 \\

\hline
\hline
Pilzer et al. \cite{pilzer2018unsupervised} & All & & & (6.400) & (0.226) & (30.20) & (3.323) & (0.842) & (0.940) & (0.975) \\

Smolyanskiy et al. \cite{Smolyanskiy_2018_CVPR_Workshops} (photo) & All  & & & - & - & 12.90 & - & - & - & - \\
Godard et al.\cite{Godard_CVPR_2017} (stereo) & All  & & & 5.742 & 0.202 & 10.80 & - & 0.928 & 0.966 &  0.980\\
Yang et al.\cite{yang2018segstereo} & All  & & & - & - & 10.03 & 1.89 & - & - & -\\
Zhou et al.\cite{Zhou_2017_ICCV} & All  & & & - & - & 9.41 & - & - & -\\
Lai et al.\cite{lai19cvpr} & All & & & 4.186, & 0.157 & 8.62 & 1.46 & 0.946 &  0.979 & 0.990\\
Yang et al.\cite{yang2018segstereo} & All  & & \checkmark & - & - & 8.79 & 1.84 & - & - & -\\
Tonioni et al. \cite{Tonioni_2017_ICCV} & &  & - & - & 8.78 & 1.48 & - & - & -\\
Li and Yuan \cite{Li2018OcclusionAS} & All  & & \checkmark & - & - & 8.21 & 1.73 & - & - & -\\
Wang et al.\cite{wang2019unos} (stereo only) & All  & & & 4.187 & 0.135 & 7.07 & - & 0.955 & 0.981 & 0.990\\
Wang et al.\cite{wang2019unos} (ego motion) & All  & & & 3.488 & 0.121 & 6.43 & - & 0.964 & 0.985 & 0.992\\
Zhong et al.\cite{ZhongArxiv2017} & All  & & & 4.857 & 0.165 & 6.42 & - & 0.956 & 0.976 & 0.985\\
Wang et al.\cite{wang2019unos} (stereo videos) & All  & & & 3.404 & 0.121 & 5.94 & - & 0.965 & 0.984 & 0.992 \\
Zhong et al.\cite{Zhong_ECCV_2018} & All  & & & (3.176) & (0.125) & (5.14) & - & (0.967) & - & -\\

\hline
\textbf{Ours} (\stereodepth MCN-BM/W-ARC) \textdagger & All & & &  3.882 &  0.117 &  4.39 & 1.07 & 0.971 &  0.988 &  0.993 \\
\textbf{Ours} (PSMNet MCN-BM/W-ARC) & All  & & &  3.764 & 0.115 & 3.85 & 1.01 & 0.974 & 0.988 & 0.993 \\
\textbf{Ours} (IResNet MCN-BM/W-ARC) & All  & & & 3.464 &  0.108 & 3.88 & 1.02 & 0.975  & 0.988 &  0.993\\
\textbf{Ours} (GwcNet MCN-BM/W-ARC) & All & & & 3.614 & 0.111 & 3.93 & 1.04 & 0.974 & 0.989 & 0.993 \\ 
\hline

\hline
Smolyanskiy et al. \cite{Smolyanskiy_2018_CVPR_Workshops} (LiDAR) & All  & \checkmark & & - & - & 15.00 & - & - & - & - \\
Smolyanskiy et al. \cite{Smolyanskiy_2018_CVPR_Workshops} (photo + LiDAR) & All  & \checkmark & & - & - & 8.80 & - & - & - & - \\
Zhou et al.\cite{Zhou_2017_ICCV} & All  & \checkmark  & & - & - & 7.29 & - & - & -\\
\hline
\end{tabular}
}
\smallskip
\caption{}
%}
\label{table:eigen}
\end{table*}
