# Supplementary material for: Reversing the cycle: self-supervised deep stereo through enhanced monocular distillation
Source: arXiv:2008.07130 source file (2020-08-17)
Supplement: Supplementary file 2 [file cityscapes_supplementary.tex]

\begin{figure}
    \centering
    \begin{tabular}{c}
        \includegraphics[width=0.5\textwidth]{images/qualitatives/cs/rgb/bremen_000089_000019_leftImg8bit.jpg} 
        \includegraphics[width=0.5\textwidth]{images/qualitatives/cs/ours/bremen_000089_000019_leftImg8bit.jpg}\\

        \includegraphics[width=0.5\textwidth]{images/qualitatives/cs/rgb/konstanz_000000_001520_leftImg8bit.jpg} 
        \includegraphics[width=0.5\textwidth]{images/qualitatives/cs/ours/konstanz_000000_001520_leftImg8bit.jpg}\\
        
        \includegraphics[width=0.5\textwidth]{images/qualitatives/cs/rgb/monchengladbach_000000_010733_leftImg8bit.jpg} 
        \includegraphics[width=0.5\textwidth]{images/qualitatives/cs/ours/monchengladbach_000000_010733_leftImg8bit.jpg}\\
        
        \includegraphics[width=0.5\textwidth]{images/qualitatives/cs/rgb/tubingen_000064_000019_leftImg8bit.jpg} 
        \includegraphics[width=0.5\textwidth]{images/qualitatives/cs/ours/tubingen_000064_000019_leftImg8bit.jpg}\\
        
        \includegraphics[width=0.5\textwidth]{images/qualitatives/cs/rgb/ulm_000069_000019_leftImg8bit.jpg} 
        \includegraphics[width=0.5\textwidth]{images/qualitatives/cs/ours/ulm_000069_000019_leftImg8bit.jpg}\\
 
         \includegraphics[width=0.5\textwidth]{images/qualitatives/cs/rgb/zurich_000002_000019_leftImg8bit.jpg} 
        \includegraphics[width=0.5\textwidth]{images/qualitatives/cs/ours/zurich_000002_000019_leftImg8bit.jpg}\\       
    \end{tabular}
    \caption{}
    \label{fig:driving_supp}
\end{figure}
