# Supplementary material for: Reversing the cycle: self-supervised deep stereo through enhanced monocular distillation
Source: arXiv:2008.07130 source file (2020-08-17)
Supplement: Supplementary file 3 [file ours_vs_guidenet_supp.tex]

\begin{table}
\centering
\begin{tabular}{l|cccc}
\hline
All  & Valid Pixels & Correct Pixels & Accuracy (\%) \\
\hline
GuideNet-LiDAR \cite{yang2019drivingstereo} \textdagger & 2,973,882 & 2,915,110 & 98.02 \\
MCN-LiDAR & 11,773,897 & 11,636,787 & 98.83 \\
MCN-BM/W-ARC & 11,551,461 & 11,247,966 & 97,37\\
MCN-SGM/L-ARC & 12,201,763 & 11,860,923 & 97.20\\
\hline
\hline
Obj & Input & Valid Pixels & Correct Pixels & Accuracy (\%) \\
\hline
GuideNet  \cite{yang2019drivingstereo} \textdagger & Stereo + LiDAR (raw) & 221,828 & 210,912 & 95.07 \\
MCN & RGB + LiDAR (raw) & 1,507,222 & 1,459,726 & 96.84 \\
MCN & RGB + WILD & 1,718,267 & 1,642,872 & 95.61\\
MCN & RGB + SGM-LRC & 1,788,154 & 1,672,222 & 93.52\\

\hline

\end{tabular}
\smallskip
\caption{\textdagger trained on LiDAR }
\label{table:guide_vs_ours}
\vspace{-10pt}
\end{table}
